# Supplementary material for: Weak phase stiffness and mass divergence of superfluid in underdoped cuprates
Source: arXiv:1005.0030 source file (2010-04-30)
Supplement: Supplementary file 1 [file Supplementary_3.pdf]

# Weak phase stiffness and mass divergence of superfluid in underdoped cuprates

Yucel Yildirim and Wei Ku

*Condensed Matter Physics and Material Science Department, Brookhaven National Laboratory, Upton, NY 11973-5000,U.S.A.*

The generalized self-consistent $T$-matrix approximation[1] is employed in this study to describe the effective interaction between the particles. The corresponding diagrammatic definition of the $T$-matrix in the Bogoliubov approximation is illustrated in Fig.1.a and in Fig.1.b.

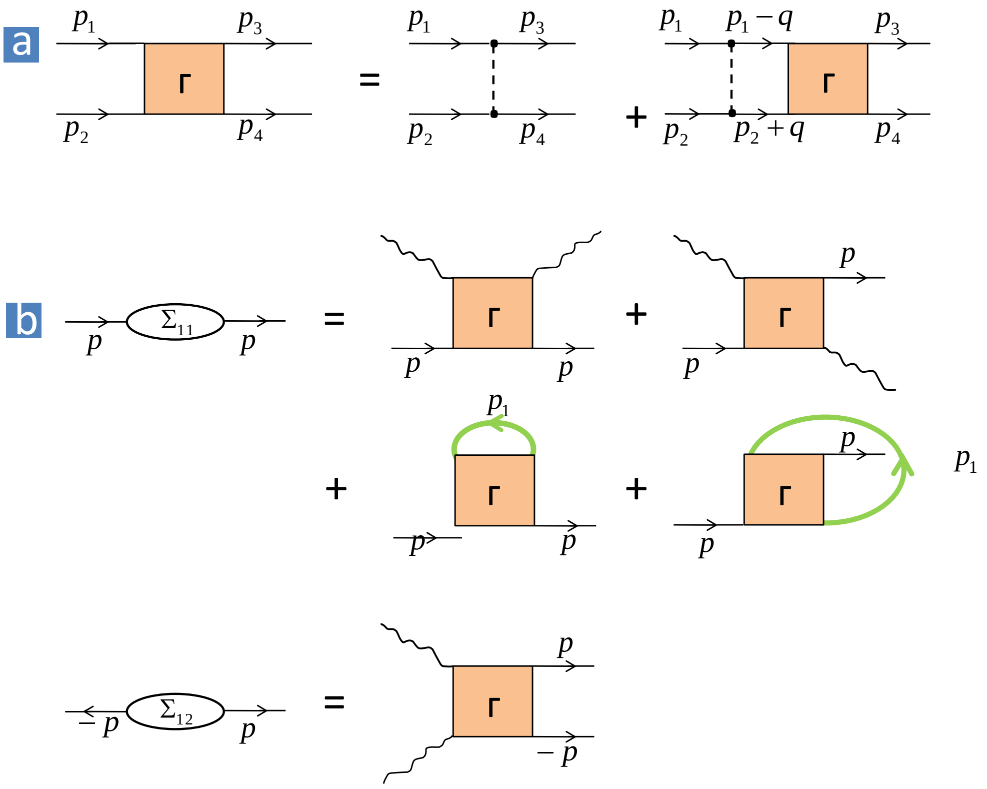


Figure 1: a) Schematic representation of the $T$-matrix $\Gamma$. b) Self-energy diagrams in the Bogoliubov approximation.

For a given scattering amplitude

$$f_0 = \frac{4\pi\hbar^2 a}{m^*} \tag{1}$$

with the effective scattering length $a$, $T$-matrix $\Gamma$ is thus[1]

$$\Gamma = \frac{f_0}{1+\alpha(T) f_0} \tag{2}$$

with $\alpha(T) = \frac{1}{V}\sum_q' [\frac{1}{\beta}\sum_{iw_l} G_{11}(\mathbf{q}, iw_l)G_{11}(-\mathbf{q}, -iw_l) - \frac{1}{2\epsilon_q}] = \int \frac{d\mathbf{k}}{(2\pi^3)}(\frac{1}{2E_k} coth(\frac{\beta E_k}{2}) - \frac{1}{2\epsilon_k})$, where $\epsilon_q$ is the bare energy of the particles.

Starting with the initial guess for $f_0$ and $\Gamma \approx f_0$ at zero temperature, the quasi-particle energy and number of particles in the condensate is evaluated via

$$E_k = \sqrt{\epsilon_k^2 + 2n_0\Gamma\epsilon_k}$$

$$n_0 = n - n_n = n - \int \frac{dw}{2}(DOS^{QP}(w)\frac{\epsilon_k + \gamma}{w}coth(\frac{\beta E_k}{2}) - DOS(w)] \quad (3)$$

where $DOS^{QP}(w)$ corresponds to quasi-particle density of states ($DOS^{QP}(w) = DOS(\epsilon)/\frac{dE}{d\epsilon}$ at $\epsilon = \sqrt{\gamma^2 + w^2} - \gamma$, where $\gamma = n_0\Gamma$) and $\beta = 1/T$. Then, $\alpha(T)$ is calculated using

$$\alpha(T) = \int dw \frac{1}{2w}[DOS^{QP}(w)coth(\frac{\beta w}{2}) - DOS(w)]. \quad (4)$$

After dropping a divergent term in Eq.4[1], Eq.2-4 are solved self-consistently until convergence is achieved. The same steps are then applied for the next (higher) temperature using the solution of the previous temperature as an initial guess.

The resulting temperature dependence of the self-consistent $T$-matrix solutions for different doppings is shown in Fig. 2. Obviously, the $T$-matrix is strongly temperature dependent. In particular, as $T \to T_c$, $\alpha(T_c) \to \infty$ and thus $\Gamma$ vanishes, in agreement with previous studies[1, 2].

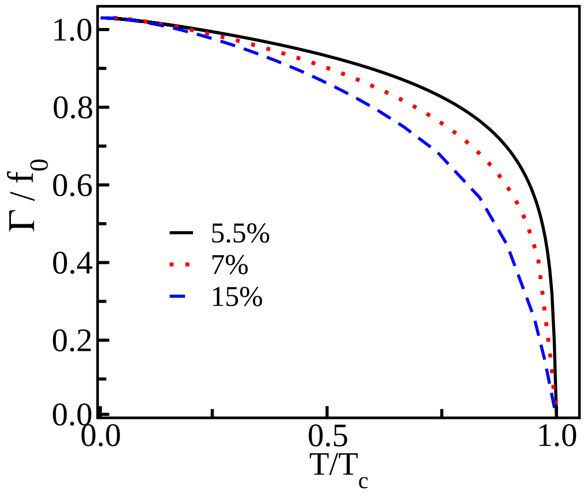


Figure 2: a) Normalized $T$-matrix as a function of T.

The vanishing of the $T$-matrix at $T_c$ allows a simple determination of $T_c$, via

$$n = n_n(T_c) = \int DOS(w)\frac{1}{e^{\beta w} - 1}dw \quad (5),$$

since in the absence of effective interactions, the system recovers the non-interacting dispersion.

# References

[1] Hua Shi & Allan Griffin Finite-tempertaure excitations in a dilute Bose-condensed gas *Physics Reports* **304**, 1–87 (1998).

[2] Bijlsma, M. & Stoof, H. T. C. Variational approach to the dilute Bose gas *Phys. Rev.A* **55**, 498–512 (1997).
